# Supplementary material for: AdaptiveCoPilot: Design and Testing of a NeuroAdaptive LLM Cockpit Guidance System in both Novice and Expert Pilots
Source: arXiv:2501.04156 source file (2025-01-07)
Supplement: Supplementary file 1 [file 9_appendix.tex]

\vspace{-0.08in}
\section{Appendix}

\begin{figure}[h!]
   \centering
   \includegraphics[width=0.95\linewidth]{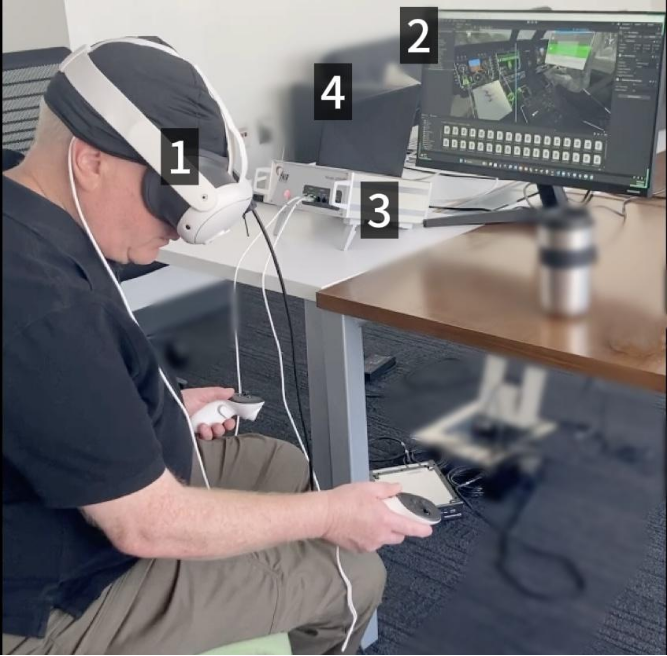}
   \caption{Apparatus. This figure shows a participant performing a trial. 1, the Quest 3 headset. 2, the experiment display for monitoring. 3, the fNIRS device. 4, the system computer.}
   \label{fig:apparatus}
\end{figure}

\begin{figure}[h!]
   \centering
   \includegraphics[width=0.95\linewidth]{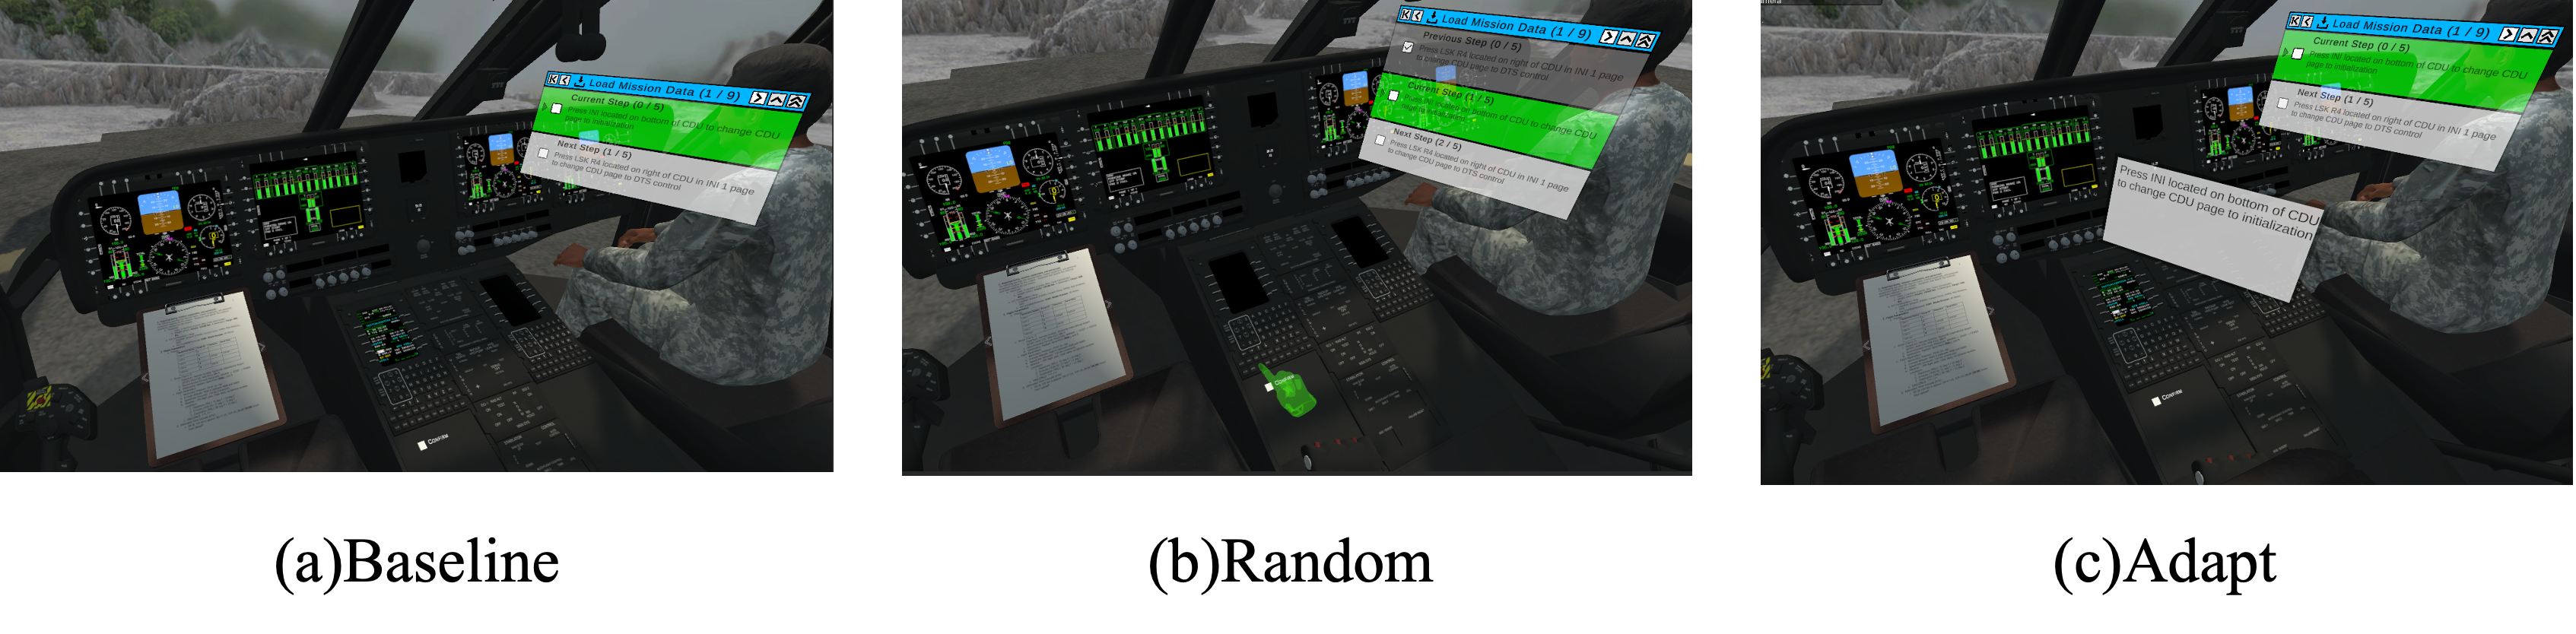}
   \caption{Experiment Condition. This figure illustrates the three conditions in our evaluation study.}
   \label{fig:evaluation_conditions}
\end{figure}

\begin{figure}[h!]
   \centering
   \includegraphics[width=0.95\linewidth]{sections/Figures/appendix/false_recognition_rates.png}
   \caption{False Error Rates. This figure shows the distribution of false errors caused by a lag in the system and the frontend.}
   \label{fig:error_distribution}
\end{figure}
